# Supplementary material for: Omni-RGPT: Unifying Image and Video Region-level Understanding via Token Marks
Source: arXiv:2501.08326 source file (2025-03-22)
Supplement: Supplementary file 1 [file video-rec-templates.tex]

\begin{table*}[!h]
\centering
\resizebox{0.98\linewidth}{!}{
\begin{tcolorbox}[colback=white!100] {
\centering
{
\begin{tabular}{p{1.0\columnwidth} c}
\begin{itemize}
\item Given the mask proposals \texttt{<mask>} in the video, can you pinpoint the one that matches \texttt{<description>},
\item From the provided masks denoted by \texttt{<mask>} in the video, which one best fits the description of \texttt{<description>},
\item Looking at the mask suggestions \texttt{<mask>} throughout the video sequence, identify the one that corresponds to \texttt{<description>},
\item In the continuous video with mask proposals \texttt{<mask>}, please highlight the one that represents \texttt{<description>},
\item Considering the mask candidates \texttt{<mask>} from multiple video frames, which one would you associate with \texttt{<description>},
\item Among the mask proposals \texttt{<mask>} seen throughout the video, can you discern the one depicting \texttt{<description>},
\item From the set of masks labeled as \texttt{<mask>} in this segment of the video, which one aligns with the description \texttt{<description>},
\item Based on the mask data provided as \texttt{<mask>} in the video, can you spot the one indicative of \texttt{<description>},
\item In the video sequence with mask suggestions \texttt{<mask>}, determine which mask resonates with \texttt{<description>},
\item Given the progression of mask proposals \texttt{<mask>} in the video, please detect the one that matches the characteristics of \texttt{<description>},
\item Reviewing the mask candidates \texttt{<mask>} from the video, can you single out the one that fits \texttt{<description>},
\item From the list of mask proposals \texttt{<mask>} appearing across the video frames, identify the one that best encapsulates \texttt{<description>},
\item Considering the provided mask data \texttt{<mask>} in the video, which one would you say corresponds to \texttt{<description>},
\item In the snapshot from the video containing mask proposals \texttt{<mask>}, please locate the mask that can be described as \texttt{<description>},
\item Based on the mask candidates \texttt{<mask>} from the continuous video sequence, can you pick the one that portrays \texttt{<description>}
\end{itemize}
\end{tabular}
}
}
\end{tcolorbox}
}

\caption{Instructions for video referring expression comprehension. We follow RegionGPT’s image referring expression template, adapted for the video domain.}
\label{tab:prompts_vidrec}
\end{table*}
